# Supplementary material for: When KV Meets Embeddings: Dynamic GPU Memory Allocation for Accelerating Generative Recommender Serving
Source: arXiv:2605.04450 source file (2026-08-24)
Supplement: Supplementary file 1 [file appendix.tex]

\section{Artifact Description (AD)}
\label{app:ad}
\textbf{Source code and components.}
The artifact includes the full \sysname{} implementation,
organized into four modules:
(1)~the three-layer RL allocator (PPO agent, OnlineAdapter, Recovery
Controller) with pre-trained checkpoints for all three datasets;
(2)~the KV--EMB-aware request scheduler with residency tracking;
(3)~the HSTU inference engine built on open-sourced HSTU~\cite{zhai2024actions}
with FBGemm~\cite{fbgemm} embedding kernels;
Baseline implementations (Static-$\alpha$, PID, XGBoost, BO, MILP,
LSTM variants) are included for comparison.
 
\textbf{Hardware and software.}
Full-scale experiments use a 32-node cluster, each equipped with
$8\times$ NVIDIA A100-80\,GB GPUs and $\geq$512\,GB CPU DRAM,
interconnected via 100\,Gbps InfiniBand EDR.
A reduced single-node configuration ($8\times$A100) is sufficient
for the allocator ablation (Table~IV, Figure~14) and single-dataset
latency experiments.
Software dependencies: Python~3.10+, PyTorch~2.1+, CUDA~12.1+,
Stable-Baselines3~2.1+, FBGemm~\cite{fbgemm},
NCCL~\cite{nccl}; Gurobi~11.0 is required only for the
MILP baseline.
 
\textbf{Datasets and preparation.}
We use three publicly available datasets:
Taobao~\cite{taobao}, Amazon Video-Games, and Amazon
Books~\cite{ni2023justifying}.
To emulate production-scale embedding memory pressure, embedding
tables are deterministically enlarged to 5\,TB using NVIDIA DLRM
synthesis scripts~\cite{dlrm_datasets}, sampling IDs from the
empirical frequency distribution to preserve the original Zipf
exponents reported in \S\ref{sec_eval_config}.
User interaction histories are extended to 8K--15K tokens via the
replay procedure described in \S\ref{sec_eval_config}.
Dataset preparation takes $\sim$2 hours and requires $\sim$6\,TB disk space.
 
\textbf{Evaluation and reproducibility.}
The automated script \texttt{run\_all.sh} executes all experiments
(3~datasets $\times$ 3~workloads $\times$ 3~seeds; $\sim$8\,h on
the full cluster, $\sim$30\,min on a single node).
Each experiment produces timestamped CSV logs recording per-window
P99 latency, QoS rate, $\alpha_t$, and cache hit rates.
A validation script \texttt{validate.py} checks that reproduced
P99 values fall within 5\% of reported means.
Plotting scripts regenerate all paper figures from logged CSVs.
Statistical reliability is ensured by repeating each configuration
with 3--5 independent random seeds and reporting mean $\pm$ 95\%
confidence intervals.
