# Supplementary material for: When KV Meets Embeddings: Dynamic GPU Memory Allocation for Accelerating Generative Recommender Serving
Source: arXiv:2605.04450 source file (2026-08-24)
Supplement: Supplementary file 2 [file tech-appendix.tex]

\section{Technical Report}
\label{app:tr}
\subsection{Latency Model and Hardware Generalization}
\label{app:latency_model}

We provide a simple cost model to answer two questions:
(1)~under what conditions does the EMB--KV dual bottleneck arise,
and (2)~does it persist on H100/H200 hardware?

\textbf{Cost model.}
A single GR request with sequence length~$L$ and $N_T$ embedding
tables incurs two $\alpha$-dependent costs:
\begin{align}
  C_{\text{emb}}(\alpha) &= \underbrace{L \cdot N_T}_{\text{lookups}}
    \cdot \underbrace{(1-h_E(\alpha))}_{\text{miss rate}}
    \cdot \underbrace{t_{\text{miss}}^{\text{emb}}}_{\text{per-miss cost}},
  \label{eq:cemb} \\[4pt]
  C_{\text{kv}}(\alpha)  &= \underbrace{(1-h_K(\alpha))}_{\text{miss rate}}
    \cdot \underbrace{\frac{4 N_L N_H d_h \, L^2}{F_{\text{gpu}}}}_{\text{full recompute}},
  \label{eq:ckv}
\end{align}
where $d{=}512$ is the embedding dimension, $F_{\text{gpu}}$ is FP16
throughput, and $N_L, N_H, d_h$ are HSTU layer/head/dimension counts.
Embedding tables are stored in fp32 ($b_e{=}4$ bytes per element)
following standard production practice, while KV tensors are stored
in fp16.

\emph{Embedding miss cost.}
On an HBM cache miss, the embedding must be fetched from CPU DRAM and from network by remote RDMA.
Since embedding tables are sharded $1/N$ across nodes
(\S\ref{sec:background}), a fraction $f_r \approx (N{-}1)/N$ of
misses target a remote shard and require an RDMA fetch before the
PCIe transfer:
\begin{equation}
  t_{\text{miss}}^{\text{emb}} =
    \frac{d \cdot b_e}{B_{\text{pcie}}}
    + f_r \cdot \frac{d \cdot b_e}{B_{\text{rdma}}}.
  \label{eq:tmiss}
\end{equation}
For $N{=}32$ nodes, $f_r \approx 0.97$; almost every HBM miss
triggers an RDMA round-trip on the critical path.
Each miss transfers $d \cdot b_e = 2{,}048$ bytes; on A100 with
100\,Gbps EDR InfiniBand, the PCIe component takes $\sim$82\,ns
and the RDMA component adds $\sim$171\,ns, making $t_{\text{miss}}
\approx 248$\,ns---roughly $3\times$ larger than a PCIe-only model
would predict.

To ground the scale: for a typical request with $L{=}10{,}000$ and
$N_T{=}10$, the total embedding volume is $\sim$200\,MB per request.
At a 90\% cache hit rate, miss traffic alone reaches $\sim$20\,MB;
at a 50\% hit rate (e.g., during cold start or popularity drift),
miss traffic exceeds 100\,MB---a significant fraction of the 30\,ms
SLO budget when transferred at an effective bandwidth of
$\sim$8\,GB/s.

\emph{KV recompute cost.}
HSTU employs encoder-level KV caching~\cite{zhai2024actions}: the
Key and Value tensors from a user's historical interaction sequence
(length~$L$) are cached in HBM so that subsequent requests for the
same user reuse them directly.
On a KV cache miss, the system must recompute the full forward pass
over the $L$-length history, dominated by self-attention:
$QK^\top$ and $\text{softmax}\cdot V$ each cost $2 N_H d_h L^2$
FLOPs per layer, yielding the $4 N_L N_H d_h L^2$ term in
Eq.~\eqref{eq:ckv}.
For the 6-layer HSTU with $d_{\text{model}}{=}512$ used in our
evaluation, a single KV miss at $L{=}10{,}000$ costs $\sim$3.9\,ms
of recomputation---over 10\% of the SLO budget.
Per-user KV tensor sizes range from $\sim$98\,MB ($L{=}8$K) to
$\sim$184\,MB ($L{=}15$K).

\textbf{Why the optimal $\alpha^*$ is interior.}
Increasing $\alpha$ grows the EMB cache, raising $h_E$ and reducing
$C_{\text{emb}}$; but it simultaneously shrinks the KV cache,
lowering $h_K$ and increasing $C_{\text{kv}}$.
The dual bottleneck exists whenever the latency-minimizing
$\alpha^*$ lies strictly inside $(0,1)$, meaning neither cache alone
should receive all HBM.
This interior optimum arises from the \emph{opposing monotonicity}
of the two costs in $\alpha$: the system must balance embedding miss
traffic against KV recomputation overhead, and the balance point
shifts with workload characteristics.

\textbf{When does the dual bottleneck arise?}
The bottleneck ratio $\Gamma = C_{\text{emb}} / C_{\text{kv}}$
governs which cost dominates at any given operating point.
Substituting and simplifying:
\begin{equation}
  \Gamma \;\propto\;
    \frac{N_T \cdot (1-h_E)}{(1-h_K) \cdot L}
    \;\times\;
    \underbrace{\frac{F_{\text{gpu}}}{B_{\text{eff}}}}_{\text{hardware ratio}},
  \label{eq:gamma}
\end{equation}
where $B_{\text{eff}} = 1/(1/B_{\text{pcie}} + f_r/B_{\text{rdma}})$
is the effective per-miss bandwidth.
When $\Gamma \approx 1$, neither bottleneck dominates and
\sysname{}'s dynamic partitioning provides the largest gains.
Three workload-level factors drive $\Gamma$:

\begin{itemize}
  \item \emph{Embedding table count $N_T$}: more tables linearly
    amplify embedding traffic.  At $N_T \leq 2$, embedding cost
    is negligible regardless of $\alpha$, yielding a KV-dominated
    regime.  Most production deployments use $N_T \in [5, 25]$.
  \item \emph{Sequence length $L$}: KV recompute scales as $L^2$
    while embedding cost scales as $L$; longer sequences shift the
    bottleneck toward KV. This is why $\alpha^*$ decreases from
    $\sim$0.50 at $L{=}2{,}048$ to $\sim$0.30 at $L{=}20{,}480$
    in~\autoref{fig_emb_kv_best_partition}.
  \item \emph{Hot-user ratio}: concentrated hot users increase
    per-node KV working-set pressure, lowering effective $h_K$.
    This is why $\alpha^*$ drops from $\sim$0.55 (Steady) to
    $\sim$0.20 (Burst) in~\autoref{fig_optimal_change}, a 0.35-wide
    swing that no static $\alpha$ can track.
\end{itemize}

Table~\ref{tab:regime} summarizes the bottleneck regimes.

\begin{table}[t]
\centering
\caption{Bottleneck regime under representative parameter settings
($d{=}512$, 6-layer HSTU, A100, $N{=}32$ nodes).
``Dual'' = interior $\alpha^*$ exists; \sysname{} provides
$>$20\% gain over best static~$\alpha$.}
\label{tab:regime}
\small
\begin{tabular}{cccc}
\toprule
$N_T$ & $h_E$, $h_K$ & $L$ & Regime \\
\midrule
1--2  & any          & any       & KV-dominated \\
3--20 & 0.80--0.98   & 2K--20K   & \textbf{Dual bottleneck} \\
$>$25 & $<$0.85      & $<$5K     & EMB-dominated \\
\bottomrule
\end{tabular}
\end{table}

The dual-bottleneck regime ($N_T \in [3,20]$, both hit rates below
0.98) covers the vast majority of production
deployments~\cite{yu2026near,gupta2020architectural,lian2022persia,
zhao2023recd}, where tens of embedding tables serve
multi-billion-item catalogs far exceeding HBM capacity.
Including the RDMA component widens this regime: the higher
effective per-miss cost means the embedding bottleneck becomes
significant even at moderately high hit rates ($h_E \sim 0.95$).

\textbf{Why it persists on H100 and H200.}
The key insight is that the hardware ratio $F_{\text{gpu}} /
B_{\text{eff}}$ in Eq.~\eqref{eq:gamma} does \emph{not} shrink
across generations.
We consider two network scenarios for H100: retaining the same
100\,Gbps EDR InfiniBand as our experimental setup, and upgrading
to 400\,Gbps NDR---the most favorable case for eliminating the
bottleneck:

\begin{table}[h]
\centering
\small
\begin{tabular}{lcccc}
\toprule
 & \textbf{A100} & \multicolumn{2}{c}{\textbf{H100}} & \textbf{H200} \\
 & \textbf{(our setup)} & \textbf{+EDR} & \textbf{+NDR} & \textbf{+NDR} \\
\midrule
$F_{\text{gpu}}$ (FP16 TFLOP/s) & 312 & 990  & 990  & 990  \\
$B_{\text{pcie}}$ (GB/s)        & 25  & 64   & 64   & 64   \\
$B_{\text{rdma}}$ (GB/s)        & 12  & 12   & 50   & 50   \\
$B_{\text{eff}}$ (GB/s)         & 8.3 & 10.4 & 28.6 & 28.6 \\
$F / B_{\text{eff}}$            & 37.7& 95.4 & 34.7 & 34.7 \\
HBM (GB)                        & 80  & 80   & 80   & 141  \\
\bottomrule
\end{tabular}
\end{table}

\noindent Two observations stand out.
First, if the network is \emph{not} upgraded alongside the GPU
(H100+EDR), $F/B_{\text{eff}}$ jumps from 37.7 to 95.4---embedding
misses become $2.5\times$ \emph{more} dominant, because compute
scales $3.2\times$ while RDMA bandwidth stays flat.
Second, even under the best-case network upgrade (H100+NDR),
$F/B_{\text{eff}}$ remains at 34.7, essentially unchanged from
A100: compute grew $3.2\times$, effective I/O bandwidth grew
$3.4\times$, keeping $\Gamma$ in the same regime.
In both scenarios, embedding misses remain a first-order latency
contributor and the dual bottleneck persists.

The H200's larger HBM (141\,GB per GPU, $\sim$1.1\,TB per 8-GPU
node) increases \emph{both} caches' capacity, but does not resolve
the zero-sum trade-off: production embedding tables (5--50\,TB)
still dwarf per-node HBM by orders of magnitude, and practical
sequence lengths (8K--15K tokens in our evaluation) yield per-user
KV sizes of $\sim$100--184\,MB, meaning even a full 8-GPU H200
node dedicating half its HBM to KV cache can hold only
$\sim$3{,}000--5{,}700 concurrent users---a small fraction of
production active user pools.
More HBM raises the absolute capacity floor but leaves the
\emph{contention} between caches intact.

\textbf{Summary.}
The EMB--KV dual bottleneck is a structural property of HSTU
inference: it arises whenever (1)~the embedding catalog far exceeds
HBM capacity, (2)~the active user pool exceeds KV cache capacity, and
(3)~multiple embedding tables amplify per-request lookup volume.
All three conditions hold in production today and are not alleviated
by newer hardware---compute-to-I/O-bandwidth ratios remain in the
same range, and embedding table / sequence length growth outpaces
HBM scaling.
Dynamic partitioning therefore remains necessary regardless of GPU
generation.

\subsection{PPO Training Details}
\label{app:ppo}
 
\textbf{Network architecture.}
The shared-backbone Actor--Critic uses a two-layer MLP with hidden
dimensions 64/128 ($<$25K parameters total).
 
\textbf{Action space parameters.}
We set the base step size $\delta = 0.02$ and allow a maximum single-step
magnitude of $k\delta$ with $k \in \{1, 2, 3\}$, yielding $\mathcal{A} = \{-3\delta,\,-2\delta,\, \delta,\,0,\,+\delta,\,+2\delta,\,+3\delta\} = \{-0.06,\,-0.04,\,-0.02,\,0,\,+0.02,\,+0.04,\,+0.06\}$. 
This design reflects the practical observation (\autoref{fig_emb_kv_partition_all})
that the optimal ratio lies within a narrow region, making fine-grained
increments are preferable to large jumps.
 
\textbf{GAE formulation.}
\begin{equation}
  \hat{A}^\text{GAE}_t =
    \sum_{l=0}^{\infty} (\gamma \lambda_\text{GAE})^l \,\delta_{t+l},
  \delta_t = r_t + \gamma V_\phi(s_{t+1}) - V_\phi(s_t).
  \label{eq:gae}
\end{equation}
GAE reduces variance relative to Monte Carlo returns at the cost of a
controlled bias, improving sample efficiency under sparse reward
signals.
 
\textbf{Replay buffer.}
Mini-batches of size 64 are sampled from a replay buffer of capacity
$B$ every $N$ steps.
The Critic is trained concurrently by minimizing the mean-squared value
error.
 
\textbf{Streaming rollouts.}
Unlike episodic training that resets the state at each epoch, we carry the
MDP state across PPO update boundaries.
This eliminates the warm-up period during which the cache is cold and
the latency baseline is miscalibrated, ensuring that every gradient
step observes a fully-warmed cache and a well-calibrated value
estimate.

\subsection{Reward Design Rationale}
\label{app:reward}
 
\textbf{Why $\gamma \approx 1$.}
A change in $\alpha$ today does not immediately manifest in the reward:
newly allocated EMB capacity must be warmed over several requests
windows before hit rates improve, and an eviction cascade triggered by
shrinking the EMB slab can suppress hit rates for multiple epochs
before the cache re-stabilizes.
Setting $\gamma \approx 1$ forces the agent to reason over these
multi-epoch propagation delays rather than myopically chasing
within-window feedback.
 
\textbf{Leading vs.\ lagging signals.}
The reward in Eq.~\eqref{eq:reward} is defined over lagging outcomes
(P99 latency, SLO violation fraction) rather than leading cache
metrics.
This is intentional: the agent should be rewarded for what it
\emph{achieves}, not for the intermediate signals it acts upon.
By contrast, P99 Lat and SLO Vio appear in the state vector to close
the feedback loop when leading signals (Hot Ratio, KV Hit, EMB Hit)
are temporarily ambiguous---e.g., during cache warm-up after a large
$\alpha$ step.
Their lower feature importance in ~\autoref{fig_important_factors} confirms
that the agent primarily acts on upstream indicators and only consults
lagging signals as a corrective signal.
 
The first term (SLO satisfaction rate) provides a dense, non-sparse
signal at every epoch and reflects the overall service quality regardless
of whether tail violations occur. The second term (tail-violation penalty proportional to severity) focuses optimization pressure on the worst-case latency that SLO contracts are defined over. Using both avoids reward hacking: optimizing only the satisfaction rate could tolerate occasional severe spikes, while optimizing only the tail penalty ignores the bulk of the request distribution.
 
\subsection{Residency Tracking Implementation}
\label{app_residency}

\textbf{KV Residency Table.}
KV cache is user-granular: each user's interaction sequence produces a
dedicated KV tensor resident on at most one node at a time. Each node
therefore maintains a \emph{KV residency table}---a hash map from user
ID to a presence bit---updated synchronously on eviction and
asynchronously on insertion (off the scheduling critical path).
At $\alpha = 0.5$, the KV pool per node is 40\,GB; at ${\sim}60$\,MB
per user (6-layer HSTU, 10K sequence length, fp16), each node holds at
most ${\sim}2k-5k$ resident KV entries, so the per-node table occupies
under 24\,KB regardless of cluster size.

\textbf{EMB Residency Table.}
Embedding cache is item-granular: the embedding table is sharded across
HBM by item ID range, and residency reflects which shards are currently
loaded. Each node maintains an \emph{EMB residency table}---a hash set
of resident shard IDs---updated synchronously on shard eviction.

\textbf{User Shard Profile.}
To evaluate EMB affinity at routing time, the scheduler precomputes
offline a \emph{user shard profile} $\mathrm{UserShardProfile}[u]$:
the top-$K$ embedding shards covering user $u$'s most-accessed items,
derived from historical interaction logs. At routing time,
$h_{\mathrm{emb}}(u, n)$ is computed as:
\begin{equation}
  h_{\mathrm{emb}}(u, n) =
  \frac{|\mathrm{UserShardProfile}[u] \cap \mathrm{EMBResidencyTable}[n]|}
       {|\mathrm{UserShardProfile}[u]|}
\end{equation}
This set intersection runs in $O(K)$ time and is performed entirely
on the router, adding negligible overhead to the scheduling critical
path. With $K = 20$ (covering ${\geq}95\%$ of per-user embedding
accesses; see \S\ref{subsec_scheduling}), the profile fits in a
small fixed-size array per user.

\textbf{Consistency Guarantees.}
The two tables are updated independently, reflecting the orthogonal
eviction policies of the KV and EMB caches. Stale residency bits
(e.g., a KV entry evicted between the routing decision and the
residency update) result in a cache miss but never in incorrect
behavior; the scheduler treats residency as a \emph{hint} rather
than a guarantee. This design cleanly separates the two cache
hierarchies and enables precise, independently-updated residency
signals for both.
